# Supplementary material for: Find a Way Forward: a Language-Guided Semantic Map Navigator
Source: arXiv:2203.03183 source file (2022-09-26)
Supplement: Supplementary file 1 [file appendix.tex]

\section{Details of landmark extraction}
\label{ap: landmark}

In landmark extraction step, we expect to extract potential landmark sequence $\langle q_i \mid q_i \in \mathcal{Q} \rangle$ from each instruction $T$. 

---- old version ----
Due to the polysemy of natural language, we design a processing pipeline to assign landmark label $q \in \mathcal{Q}$ to 
%potential landmark 
noun word $w_j \in T$ based on WordNet. We first manually annotate the synset of each landmark label $q \in \mathcal{Q}$ based on definitions in WordNet. We denote the mapper of the object label $q$ to its synset as $\mathbf{S}_{obj}$. 
%For each instruction $T$, we extract potential landmarks first by identifying possible object words such as ``oven" and ``table". To do so, we apply part-of-speech (POS) tagging on $T$ and select all noun tokens to construct candidate list $\mathbf{W} = \{w_i\}_{i=1}^{n}$.
We selects all nouns by applying part-of-speech (POS) tagging on each $T$ to form a candidate word list  $\mathbf{W} = \{w_i\}_{i=1}^{n}$.
Then we apply Word Sense Disambiguation (WSD) with Lesk algorithm [cite] % might switch to T5 
on each noun $w_i$ to identify its synset $s_i$ in the context of $T$.
\begin{equation}
    s_i = \text{WSD}(w_i, T)
\end{equation}
We use synset-level WuPalmer similarity [cite] to measure matching score between $w_i$ and each landmark label $q$ in $\mathcal{Q}$. The similarity score measures how close this two synsets in the WordNet tree. The closest matching landmark label $\tilde{q}_i$ is chosen by 
\begin{equation}
    \tilde{q}_i = \argmaxA_{q \in \mathcal{Q}} \text{WuPalmer}(s_i, \mathbf{S}_{obj}(q))
\end{equation}
Since irrelevant nouns can also appear in candidates, we filter the candidates with a thresholding factor of $\gamma=0.85$ to extract only candidates close to synsets in $\mathbf{S}_{obj}$. Then we get potential landmark sequence $X = \langle \tilde{q}_i \mid \text{WuPalmer}(s_i, \mathbf{S}_{obj}(\tilde{q}_i)) > \gamma \rangle$

\section{Pattern design for moving action recognition}
\label{ap: action}
For instance, ``turn right" is a key component for path proposing, but it has many alternatives in natural language such as ``take a right turn" or ``head to the right". These alternatives usually share the same syntax rule, such as before the keyword ``right" it will have a verb with some modifiers. On the other hand, the syntax rule should also avoid phrase not describing a moving action, such as ``can observe a picture on the right wall". We design patterns for ``turn left" and ``turn right" to help the moving action recognition, for the details please refer to Appendix.~\ref{ap: action}. 

\section{Compare to vln task}
\begin{table*}[t]
\centering
    \begin{threeparttable}
        \begin{tabular}{AA BBBBBB BBBBBB}
        \toprule
         & \multirow{2}{*}{\textbf{Model}} & \multicolumn{6}{c}{\textbf{Val\_Seen}} & \multicolumn{6}{c}{\textbf{Val\_Unseen}}  \\
        \cmidrule(lr{1em}){3-8}  \cmidrule(lr{1em}){9-14} 
        & & TL $\downarrow$ & NE $\downarrow$ & nDTW $\uparrow$ & OS $\uparrow$ & SR $\uparrow$ & SPL $\uparrow$ &  TL $\downarrow$ & NE $\downarrow$ & nDTW $\uparrow$ & OS $\uparrow$ & SR $\uparrow$ & SPL $\uparrow$  \\
        \midrule
        
        RGBD &
        \textbf{Seq2Seq-DA-full} &  \\
        
        & \textbf{CMA-DA-PM-Aug-full} & \\
        & \textbf{WPN + DN} & 9.52 & 6.23 & - & 0.45 & 0.37 & 0.33 & 9.86 & 6.93 & - & 0.40 & 0.33 & 0.29 \\
        & \textbf{HPN + DN} & 8.54 & 5.48 & - & 0.53 & 0.46 & 0.43 & 7.62 & 6.31 & - & 0.40 & 0.36 & 0.34 \\
        
        \midrule
        
        Map & \textbf{Seq2Seq-DA-Map} & 9.73 & 8.31 & 0.45 & 0.38 & 0.26 & 0.24 & 9.47 & 8.55 & 0.41 & 0.31 & 0.21 & 0.18 \\
        & \textbf{CMA-DA-PM-Aug-Map} &  &  &  &  &  &  &  &  &  &  &  & \\
        
        \midrule
        
        & \textbf{ours*}  & 8.61 & 5.75 & 0.63 & 0.53 & 0.44 & 0.42 & 7.75 & 6.07 & 0.61 & 0.46 & 0.39 & 0.37 \\
        % & \textbf{ours*}  & - & - & - & - & 0.48 & - & - & - & - & - & 0.36 & - \\
        \bottomrule
        \end{tabular}
    \begin{tablenotes}
    \item * stands for models trained only on iPPD splits (single floor large environment), others are validation results of official checkpoints on the iPPD validation split.
    \end{tablenotes}
\end{threeparttable}
\caption{Performance in iPPD. We find even with smaller training set, navigation on map with our proposed method outperform others on seen environment. In the meantime, our method has comparable performance for NE and nDTW on unseen environment with SOTA method~\cite{krantz2021waypoint}. 
% NOTE: val\_unseen contains smaller single\-floor scenes but has height changes 
} 
\label{tab: main old}
\end{table*}
